# Supplementary material for: Monotone Ecological Inference
Source: arXiv:2504.14752 source file (2025-04-20)
Supplement: Supplementary file 1 [file analysis_of_framework.tex]

\subsection*{Bounds}

\subsection*{Inference}
We now describe strategies for inference, particularly for confidence intervals, of our primary methods. For the regression estimator, because the estimator is equivalent to and recovered from the coefficient in a regression model, and it is known that ordinary least squares regression is consistent and asymptotically normal, we can use straightforward p-values and confidence intervals as normally practiced. Note that the confidence interval obtained is not of $D$, but of $D^r$, i.e. the coefficient. For the weighted estimator, we note that:
\begin{align*}
    \widehat{D}_n^w = \frac{\sum(b_i-\bar{b})^2}{\bar{b}(1-\bar{b})} \widheat{D}_n^r &\implies\\ \Var\left(\widehat{D}_n^w|b\right)& = \left(\frac{\sum(b_i-\bar{b})^2}{\bar{b}(1-\bar{b})}\right)^2 \Var \left(\widehat{D}_n^r|b\right)
\end{align*}
Given the data, this allows us to recover the standard error of $\widehat{D}_n^w$  as a multiplicative factor of the standard error $\widehat{D}_n^r$, and thus construct confidence intervals in the same way. 

For large enough data, we may approximate these confidence intervals by the standard error of the asymptotic regime. The following theorem provides the asymptotic behavior of $\widehat{D}_n^w$:

\begin{thm}\label{thm:asympt}
The sampling distribution of $\widehat{D}_n^w$ converges to:
\begin{align*}
 \widehat{\mathcal{D}}_{n}^w \longrightarrow \mathcal{N}\left(D^w, \frac{\sigma^2}{n \E[b^2]}\frac{\Var(b)}{\E[b](1-\E[b])}\right)
\end{align*}
\end{thm}

In the case that both covariance terms are of positive sign, a (naive) confidence interval can be constructed by as:
\begin{definition}[Naive Confidence Interval]
Given $b$ and the estimators above, a $1-\alpha/2$ confidence interval is given by:
\begin{align*}
    \text{CI}^{\alpha}:=\left[\widehat{D}_n^w - \widehat{\text{SE}}^{w} \cdot z_{\alpha/2}, \widehat{D}_n^r + \widehat{\text{SE}}^r \cdot  z_{\alpha/2}\right]
\end{align*}
where $z_{\alpha/2}$ is the standard normal distribution inverse of $1-\alpha/2$ and $\widehat{SE}_n^w$ and $\widehat{SE}_n^r$ are the estimated standard errors of $\widehat{D}_n^w$ and $\widehat{D}_n^r$, respectively. 
\end{definition}
A similar definition can be made for the case that the signs of both covariance terms is negative. 

However, one may note that these confidence intervals may be too wide, as they treat the two estimators as if they were entirely unrelated. 

\subsection*{Implications for Methodology}
We briefly highlight the implications of these results for the problem of creating a coherent framework. For any ecological-inference-type problem, we thus can obtain bounds on the relationship of interest if the conditions of points 3 and 4 in Theorem \ref{thm:bounds} hold.
